# Supplementary material for: Eigenvalue crossing as a phase transition in relaxation dynamics
Source: arXiv:2209.09307 ancillary file (2022-09-19)
Supplement: Supplementary file 1 [file SM.pdf]

# Supplemental Material for :"Eigenvalue crossing as a phase transition in relaxation dynamics"

Gianluca Teza, Oren Raz, and Oren Raz[a)]
*Department of Physics of Complex Systems, Weizmann Institute of Science, Rehovot 7610001, Israel*

(Dated: 19 September 2022)

In this supplemental material (SM) we discuss the details of the calculations and results presented in the main text, as well as additional models supporting our analyses and conclusions.

## I. MINIMAL SETUP FOR LEVEL CROSSING IN A MARKOVIAN SYSTEM

In this section we prove that in a 3-state Markovian system the phenomenon of eigenvalue crossing, with respect to the bath temperature $T_b$, cannot occur. Following the characterization of the manuscript, we use the Arrhenius form as a general formulation of the rate matrix $R^1$:

$$R_{ij}(T_b) = \begin{cases} \Gamma e^{-(B_{ij}-E_j)/T_b} & i \neq j \\ -\sum_{k\neq i} R_{ki} & i = j \end{cases} \tag{1}$$

where $\Gamma$ (= 1 for simplicity) is a rate constant and $B_{ij} = B_{ji}$ denotes the energy barrier between state $i$ and $j$, set to be higher than the adjacent energy levels $E_{\{i,j\}}$, in units in which $k_B = 1$. For finite values of energies and barriers, this formulation grants that the system is ergodic and that in the long time limit it relaxes towards the Boltzmann equilibrium $\pi_i(T_b) \propto e^{-E_i/T_b}$. The rate matrix can be decomposed as:

$$R = VDV^{-1} \tag{2}$$

where $D_{ij} = \delta_{ij}\lambda_i$ is a diagonal matrix containing the eigenvalues $0 = \lambda_1 < \lambda_2 \leq \lambda_3$ (due to ergodicity and detailed balance), while $V_{ij} = (\vec{v}_j)_i$ and $V^{-1}_{ij} = (\vec{u}_i)_j$ are the right and left eigenvectors matrices, respectively.

Assuming a crossing at a certain bath temperature $T^*$, we get that $\lambda_2(T^*) = \lambda_3(T^*) \equiv \lambda$, implying

$$\begin{aligned} R_{ij}(T^*) =& \sum_{kl} V_{ik}(T^*) \begin{pmatrix} 0 & 0 & 0 \\ 0 & -\lambda & 0 \\ 0 & 0 & -\lambda \end{pmatrix}_{kl} V^{-1}_{lj}(T^*) \\ =& \sum_{kl} \lambda V_{ik}(T^*) \left(\delta_{1k}\delta_{1l} - \delta_{kl}\right) V^{-1}_{lj}(T^*) \\ =& \lambda \left(V_{i1}(T^*)V^{-1}_{1j}(T^*) - \delta_{ij}\right) = \lambda \left(\pi_i(T^*) - \delta_{ij}\right) \end{aligned} \tag{3}$$

where we exploited the fact that the first right and left eigenvectors are the Boltzmann equilibrium and unit vector, respectively. According to the Arrhenius formulation of the rates (Eq. 1), we see that the rates have an exponential dependence on the bath temperature. This allows us to express any off-diagonal term at a general temperature as $R_{ij}(T_b) = R_{ij}(T^*)^{T^*/T_b}$, while the diagonal ones simply are determined by imposing a zero sum on the columns for probability conservation. Consequently, one finds that for any temperature

$$R_{ij}(T_b) = \lambda^{T_b/T^*} \left(\pi(T^*) - \delta_{ij}\right) \tag{4}$$

---

a) Electronic mail: oren.raz@weizmann.ac.il

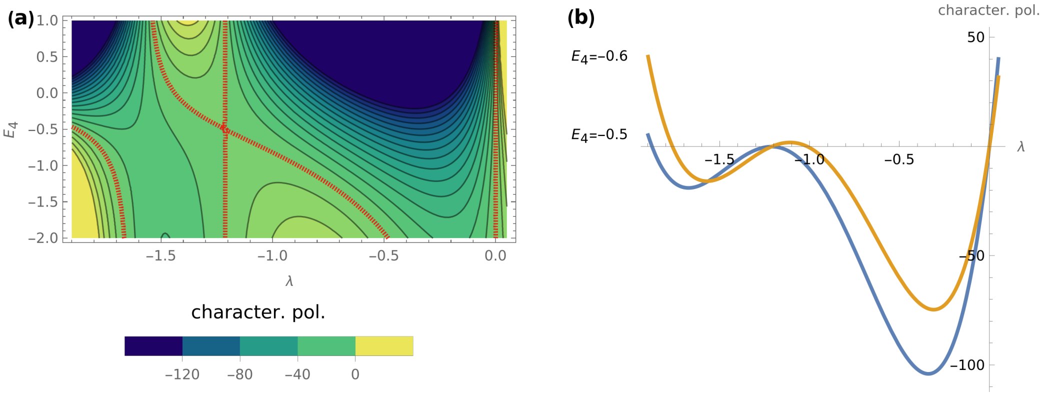


FIG. 1. (a) Characteristic polynomial of the eigenvalues of the 4-state system exhibiting level crossing, as a function of the parameter determining the eigenvalues ($\lambda$) and the energy of the fourth well $E_4$. The red dashed line highlights the zero contour line, indicating the roots of the polynomial. It is clear how at $E_4 = -1/2$ the second and third eigenvalues become degenerate, providing a crossing, while for any other value of $E_4$ the roots are all distinct. (b) Characteristic polynomial plotted in the case of eigenvalue crossing ($E_4 = -1/2$, blue line) and the avoided crossing example presented in the main text ($E_4 = -0.6$, yellow line).

implying that the eigenvalues themselves inherit the trivial exponential dependence on temperature from the rates. Therefore, the degeneracy we imposed for $T^*$ holds at all bath temperatures, finally proving the initial argument. An analogous proof follows for the general case of a $N$-state system exhibiting a degeneracy of order $N-1$ in the second eigenvalue.

## II. LEVEL CROSSING IN A 4-STATE SYSTEM

A 4-state Markovian model is the minimal setup that can allow to observe a level crossing. The characteristic polynomial of the eigenvalues of such a system is of third order, but we are ensured that all roots are real given the properties of the rate matrix which we built according to the Arrhenius formalism (Eq. 1). The number of free parameters of this setup is 10, while we have only one constraint for an eigenvalue crossing at some $T^*$, which is the second and third eigenvalues to match at that temperature, meaning $\lambda_2(T^*) = \lambda_3(T^*)$. Therefore we can reduce the number of free parameters to 2 in order to retain an explicit analytic solution that characterizes the crossing. We therefore set $E_1 = -1$, two degenerate wells $E_2 = E_4$ with an infinite barrier $B_{24} = +\infty$ dividing them, and we set all the other barriers to 0 height. This choice provides us with the following rate matrix:

$$R(T_b) = \begin{pmatrix} -3e^{-1/T_b} & e^{E_4/T_b} & e^{E_3/T_b} & e^{E_4/T_b} \\ e^{-1/T_b} & -2e^{E_4/T_b} & e^{E_3/T_b} & 0 \\ e^{-1/T_b} & e^{E_4/T_b} & -3e^{E_3/T_b} & e^{E_4/T_b} \\ e^{-1/T_b} & 0 & e^{E_3/T_b} & -2e^{E_4/T_b} \end{pmatrix} \tag{5}$$

with eigenvalues

$$\begin{aligned} \lambda_1 &= 0 \\ \lambda_2 &= -2e^{\frac{E_4}{T_b}} \\ \lambda_{3,4} &= \frac{1}{2}\Bigg( -3e^{\frac{E_3}{T_b}} - 2e^{\frac{E_4}{T_b}} - 3e^{-\frac{1}{T_b}} + \\ &\pm\sqrt{-4e^{\frac{E_3+E_4}{T_b}} - 14e^{\frac{E_3-1}{T_b}} + 9e^{\frac{2E_3}{T_b}} - 4e^{\frac{E_4-1}{T_b}} + 4e^{\frac{2E_4}{T_b}} + 9e^{-\frac{2}{T_b}}}\Bigg) \end{aligned} \tag{6}$$

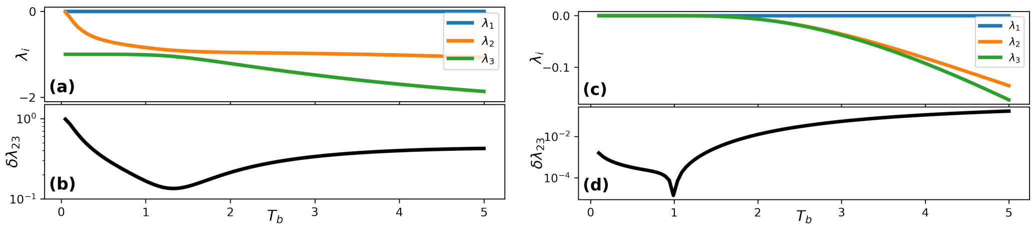


FIG. 2. (a,b) Eigenvalues and eigenvalue difference of the fully connected 3-state model with parameters taking the values shown in Eq. 9. The system exhibits avoided crossing between the second and third eigenvalues at $T^* = 1$. (c,d) Same as above, only for a 3-state chain (the values of the parameters are shown in Eq. 10). The avoided crossing is present also in this case.

Imposing a crossing at bath temperature $T^* = 1$ we get after straightforward calculation that the following relationship between the remaining free parameters must hold:

$$E_3 = \log \frac{e^{E_4}}{4 - e^{1+E_4}} \text{ for } E_4 < -1 + 2\log 2 \tag{7}$$

which for $E_4 = -1/2$ (example provided in the manuscript) provides us with a crossing if $E_3 = -\log(4\sqrt{e} - e) \simeq -1.35$. An analysis of the characteristic polynomial shows that its determinant becomes strictly greater than zero as soon as any parameter is perturbed. As an example, breaking the degeneracy among the two same-depth wells $E_2$ and $E_4$ will immediately introduce an additional real zero in such polynomial, which translates in the avoided crossing showed in the main text (see Fig. 1).

## III. AVOIDED CROSSING IN A 3-STATE SYSTEM

Even though we showed that a crossing cannot happen in a 3-state Markovian setup, this doesn't exclude the possibility of observing avoided crossing. In this scenario, the two eigenvalues regulating the slowest dynamics can approach arbitrarily close to one another without ever crossing. Such phenomena can be monitored through the relative difference between them, defined as $\delta\lambda_{23} = -(\lambda_2 - \lambda_3)/\lambda_3$, which exhibits a minimum at the avoided crossing temperature $T^*$. Indeed, numerical analyses allowed us to easily find systems that are characterized by such property.

Following the general Arrhenius formulation introduced above (Eq. 1), we can explicitly find the second and the third eigenvalue as the roots of the second order characteristic polynomial. We find that:

$$\begin{aligned}
\lambda_{2,3}(T_b) = -\frac{1}{2}\Bigg( & e^{-\frac{B_{23}+E_2}{T_b}} + e^{-\frac{B_{23}+E_3}{T_b}} + e^{-\frac{B_{13}+E_3}{T_b}} + e^{-\frac{B_{13}}{T_b}} + e^{-\frac{B_{12}+E_2}{T_b}} + e^{-\frac{B_{12}}{T_b}} + \\
& \pm\Bigg[\left(e^{-\frac{B_{23}+E_2}{T_b}} + e^{-\frac{B_{23}+E_3}{T_b}} + e^{-\frac{B_{13}+E_3}{T_b}} + e^{-\frac{B_{13}}{T_b}} + e^{-\frac{B_{12}+E_2}{T_b}} + e^{-\frac{B_{12}}{T_b}}\right)^2 + \\
& -4\left(e^{\frac{E_2+E_3}{T_b}} + e^{E_2/T_b} + e^{E_3/T_b}\right) e^{-\frac{B_{12}+B_{13}+B_{23}}{T_b}} \left(e^{B_{12}/T_b} + e^{B_{13}/T_b} + e^{B_{23}/T_b}\right)\Bigg]^{1/2}\Bigg)
\end{aligned} \tag{8}$$

Then, we can exploit an optimization algorithm[2] to maximize the difference between the two derivatives $\partial_{T_b}(\lambda_2 - \lambda_3)$ at a temperature $T^* + \Delta T$ slightly above the crossing one, while requiring a small difference between the eigenvalues at $T^*$ as a constraint. In Fig. 2a,b we report the example of a configuration obtained with this procedure exhibiting an avoided crossing at $T^* = 1$, for the following parameters (the amplitude is an irrelevant parameter in this analysis, which we set to $\Gamma \equiv 1$):

$$E_1 = 0 \ , \ E_2 = 0.9 \ , \ E_3 = -15 \ , \ B_{12} = 3.8 \ , \ B_{23} = 1.1 \ , \ B_{13} = 0.1 \tag{9}$$

It is also important to mention how we were able to obtain an avoided crossing for an even simpler case, namely a 3-state chain. This setup corresponds to the case in which a barrier (e.g. $B_{13}$) is infinitely high, making the jumps between two states impossible and therefore breaking periodicity in the system. Following the same procedure described above for this configuration we obtain an avoided crossing at $T^* = 1$ with the following paraemters:

$$E_1 = 0 \ , \ E_2 = -19.89 \ , \ E_3 = -7.1 \ , \ B_{12} = 8.2 \ , \ B_{23} = 1.1 \ , \ B_{13} = +\infty \tag{10}$$

Although the crossing itself is less visible, as we can see in Fig. 2c,d, it has an important experimental relevance as a non-periodic configuration was recently used in colloidal setups to prove the Mpemba effect[3] and its inverse[4].

[1]D. Mandal and C. Jarzynski, "A proof by graphical construction of the no-pumping theorem of stochastic pumps," Journal of Statistical Mechanics: Theory and Experiment **2011**, P10006 (2011).
[2]In this case we used the Sequential Least Squares Programming (SLSQP) algorithm from the SciPy Pyhton library. For a reference see here.
[3]A. Kumar and J. Bechhoefer, "Exponentially faster cooling in a colloidal system," Nature (2020).
[4]A. Kumar, R. Chétrite, and J. Bechhoefer, "Anomalous heating in a colloidal system," Proceedings of the National Academy of Sciences **119** (2022).
